# Supplementary material for: Functional Variational Bayesian Neural Networks
Source: arXiv:1903.05779 source file (2019-03-14)
Supplement: Supplementary file 1 [file appendix-functional-vi.tex]

\section{Function-Space Inference versus Weight-Space Inference}
In this section, we compare function-space inference with weight-space inference. 
We study the setting that we have a weight-space prior which matches the functional prior in function space. Despite that prior is not a problem anymore under this setting, we show that performing inference in function space is still superior to performing inference in weight space.

Consider a deep linear network with weights $\{\bW_{l}\}_{l=1}^{L-1}$, 
the network defines a function:
\begin{align}
    f(\bx) = \bW_{L-1} \cdots \bW_{1} \bW_{0} \bx = \prod_{l=0}^{L-1} \bW_{l} \bx =: \mathcal{W} \bx
    \end{align}

Given dataset $\mathcal{D}=(\bX^{\data}, \by^{\data})$ and weight-space prior $p_w(\bW_0, \cdots , \bW_{L-1})$, variational inference is adopted to approximate the intractable posterior.

{\bf Weight-Space Variational Inference.} Assuming a variational posterior $q_w(\bW_0, \cdots , \bW_{L-1})$,
\begin{align}\label{eq:linear-weight}
    \elbo_w = \mathbb{E}_{q_w} \log p(\by^{\data} | \bX^{\data}, \prod_{l=0}^{L-1} \bW_{l} ) - \KL{q(\begin{bmatrix}\bW_0, \cdots , \bW_{L-1} \end{bmatrix})}{p(\begin{bmatrix}\bW_0, \cdots , \bW_{L-1} \end{bmatrix})}
\end{align}
{\bf Function-Space Variational Inference.} Because $f(\bx) = \prod_{l=0}^{L-1} \bW_{l} \bx =: \mathcal{W} \bx$, the weight-space prior $p_w$ corresponds to a prior $p_{\mathcal{W}}(\mathcal{W})$, thus corresponds to a functional prior $p_f(f)$. Similarly, the weight-space variational posterior $q_w$ corresponds to a prior $q_{\mathcal{W}}(\mathcal{W})$, thus corresponds to a functional prior $q_f(f)$.  

Consider the functional variational inference, 
\begin{align}
    \elbo_f &= \mathbb{E}_{q_f} \log p(\by^{\data} | \bX^{\data}, f) - \KL{q_f(f)}{p_f(f)} \\
    &= \mathbb{E}_{q_w} \log p(\by^{\data} | \bX^{\data}, \prod_{l=0}^{L-1} \bW_{l} )  - \KL{q_f(f)}{p_f(f)} 
\end{align}

\begin{thm}[ELBO Ordering]\label{thm:elbo-order} The functional ELBO is no smaller than the weight-space ELBO.
\begin{align}
    \elbo_f \geq \elbo_w
\end{align}
\end{thm}
%\begin{rem} Using independent priors $p(\bW_0, \cdots \bW_{L-1})=\prod_{l=0}^{L-1}p(\bW_l)$, variational inference under factorized distributions $q(\bW_0, \cdots \bW_{L-1})=\prod_{l=0}^{L-1}q(\bW_l)$ can induce big gap $\elbo_f - \elbo_w$, because the KL term in \Cref{eq:linear-weight} expands to multiple additions.
%\end{rem}

\begin{lem}[Linear Processes KL Divergence]\label{lem:linear-kl} Consider functions $f(\bx)=\mathcal{W} \bx : \mathbb{R}^d \rightarrow \mathbb{R}^o$ and two distributions $p_{\mathcal{W}}(\mathcal{W}), q_{\mathcal{W}}(\mathcal{W})$. Equivalently, the two distributions correspond to function distributions $p_f(f), q_f(f)$, respectively. Then the functional KL divergence 
\begin{align}
    \KL{q_f(f)}{p_f(f)} = \KL{q_{\mathcal{W}}(\mathcal{W})}{p_{\mathcal{W}}(\mathcal{W})}
\end{align}

\end{lem}

\begin{proof}[Proof of \Cref{{lem:linear-kl}}] By \Cref{thm:kl}, the functional KL divergence is given by the supremum over all finite sets of input locations,
\begin{align}
    \KL{q_f(f)}{p_f(f)} &=  \underset{n, \bx_{1:n}}{\sup} \KL{q(\bbf_{\bx_{1:n}})}{p(\bbf_{\bx_{1:n}})} \notag  \\ 
    &= \underset{n, \bx_{1:n}}{\sup} \KL{q([
\mathcal{W} \bx_1 ,
\cdots 
\mathcal{W} \bx_n ]
)}{p([
\mathcal{W} \bx_1 ,
\cdots 
\mathcal{W} \bx_n ])} \notag  \\
&= \underset{n, \bx_{1:n}}{\sup} \KL{q_{\mathcal{W}}(\mathcal{W})}{p_{\mathcal{W}}(\mathcal{W})} \notag\\
&= \KL{q_{\mathcal{W}}(\mathcal{W})}{p_{\mathcal{W}}(\mathcal{W})}
\end{align}
Where the second last equation comes from the bijection between $\mathcal{W} $ and $[
\mathcal{W} \bx_1 ,
\cdots 
\mathcal{W} \bx_n ]$, where KL divergence keeps unchanged with bijection mapping (In rare cases $\bx_{1:n}$ don't have sufficient rank to support a bijection, the KL is smaller than $\KL{q_{\mathcal{W}}(\mathcal{W})}{p_{\mathcal{W}}(\mathcal{W})}$ thus diminishes with $\sup$).
\end{proof}

\begin{proof}[Proof of \Cref{thm:elbo-order}] Based on \Cref{lem:linear-kl}, the functional ELBO
\begin{align}
    \elbo_f 
    &= \mathbb{E}_{q_w} \log p(\by^{\data} | \bX^{\data}, \prod_{l=0}^{L-1} \bW_{l} )  - \KL{q_f(f)}{p_f(f)}  \notag \\
    &= \mathbb{E}_{q_w} \log p(\by^{\data} | \bX^{\data}, \prod_{l=0}^{L-1} \bW_{l} )  - \KL{q_{\mathcal{W}}(\mathcal{W})}{p_{\mathcal{W}}(\mathcal{W})}  \notag \\
    &\geq \mathbb{E}_{q_w} \log p(\by^{\data} | \bX^{\data}, \prod_{l=0}^{L-1} \bW_{l} )  - \KL{q(\begin{bmatrix}\bW_0, \cdots , \bW_{L-1} \end{bmatrix})}{p(\begin{bmatrix}\bW_0, \cdots , \bW_{L-1} \end{bmatrix})}  \notag \\
    &= \elbo_w  \notag 
\end{align}
Where the inequality stems from the fact that $\mathcal{W}=\prod_{l=0}^{L-1} \bW_{l}$.
\end{proof}

\begin{exampp}[Deep Addition Networks]
Similar to deep linear networks, deep addition networks performs addition in each layer, thus it defines the function $f: \mathbb{R} \rightarrow \mathbb{R}$ that 
\begin{align}
    f(x) = x + w_0 + \cdots + w_{L-1} = x + \sum_{l=0}^{L-1} w_l =: x + w
\end{align}
Consider Gaussian weights prior $p_w^l(w_l)=\mathcal{N}(0, \frac{\eta^2}{L}), l=0: L-1$, and Gaussian weights variational posterior $q_w^l(w_l)=\mathcal{N}(\mu_l, \sigma_l^2), l=0 : L-1$. They are equivalent to the prior $p_w(w)=\mathcal{N}(0, \eta^2)$ and the variational posterior $q_w(w)=\mathcal{N}(\sum_l \mu_l, \sum_l \sigma_l^2)$. The likelihood term is 
\begin{align}
    y = \mathcal{N}(f(x), \nu^2)
\end{align}

Assume we have a dataset $\data = \{(x_i, y_i)\}_{i=1}^n$,

{\bf Function-Space Inference} The exact posterior over $w$ is a Gaussian distribution, the same as $q_w(w)$. Therefore the optimal variational posterior using functional inference is the true posterior 
\begin{align} \label{eq:deep-addition-func-q}
    p(w|\data) = \mathcal{N}(\frac{\eta^2 \sum_i (y_i-x_i)}{n\eta^2 + \nu^2}, \frac{\nu^2 \eta^2}{n\eta^2 + \nu^2})
\end{align}
{\bf Weight-Space Inference} Under factorized Gaussian variational posterior, we can get the optimal $q_w^l$ as 
\begin{align}
    q_{w}^{ l \star}(w_l) = \mathcal{N}(\frac{1}{L}\frac{\eta^2 \sum_i (y_i-x_i)}{n\eta^2 + \nu^2}, \frac{\nu^2 \eta^2}{n\eta^2 + L \nu^2 })
\end{align}
Therefore, the aggregated $w$ distribution using weight-space inference becomes 
\begin{align}\label{eq:deep-addition-weight-q}
    q_{w}^{\star}(w) = \mathcal{N}(\frac{\eta^2 \sum_i (y_i-x_i)}{n\eta^2 + \nu^2}, \frac{\nu^2 \eta^2}{ n \eta^2 / L  + \nu^2 })
\end{align}
\Cref{eq:deep-addition-weight-q} and \Cref{eq:deep-addition-func-q} have the same mean, but different covariances. Considering using deeper networks for weight-space inference, $\nu^2$ will finally dominate $n\eta^2 / L$. In the limit that $L \rightarrow \infty$, the variance will become prior variance.
\end{exampp}
